# Supplementary material for: CommRad: Context-Aware Sensing-Driven Millimeter-Wave Networks
Source: arXiv:2407.08817 source file (2024-07-11)
Supplement: Supplementary file 1 [file appendix.tex]

\appendix

\section{Constructive Multi-beam is optimal for SNR and throughput for general k-path channel}\label{appendix:A}
Here we show that the multi-beam patterns with appropriate power and phase control are optimal such that they maximize the SNR at the receiver. To demonstrate the multi-beam optimality, we first construct the maximum likelihood (ML) based solution and then show that the multi-beam approaches the ML estimate. Recall the optimal beamforming weights for a general multi-path channel $\hbf$ is given by:

% The transmit phased array applies beam weights $\wbf_T$ to transmit signal $s[m]$ which then passes through channel $\hbf$. For simplicity, assume a single antenna at the receiver with a receive antenna gain of unity. The received signal $y[m]$ corrupted with noise $n[m]$ ($m$ is symbol index) as follows:

% \begin{equation}
%     \begin{split}
%         y[m] = \hbf^T \wbf_T s[m] + n[m].
%     \end{split}
% \end{equation}

% % where, 

% % \begin{equation}
% %     \begin{split}
% %         h_{\text{eff}} = \wbf_R^H \Hbf \wbf_T
% %     \end{split}
% % \end{equation}

% We write the expression of SNR:
% \begin{equation}
% \begin{split}
%       \text{SNR} &= \frac{||\hbf^T \wbf_T ||^2 P_T}{P_N},
%       %&= \sum_{\ell=1}^L ||\abf_T(\phi_\ell)\wbf_T||^2 ||\gamma_\ell||^2 \frac{P_T}{P_N} 
% \end{split}
% \end{equation}
% where $P_T = \sum_m{||x[m]||^2}$ is the average transmit power (without transmit antenna gain) and $P_N$ is the noise power.

% The optimal linear ML estimator for $\wbf_T$ is given by
% \begin{equation}
%     \begin{split}
%         \hat{\wbf}_T &= \argmax_{\wbf_T} \text{SNR}\\
%         &\text{s.t. } ||\wbf_T||=1,
%     \end{split}
% \end{equation}
% where the constraint $||\wbf_T||=1$ normalizes the transmit beam pattern to satisfy the total radiated power constraint. The ML estimate of optimal beam weights is
\begin{equation}\label{eq:wmrc2}
    {\wbf}^{\text{opt}}  = \frac{\hbf^*}{||\hbf||},
\end{equation}
which provides the maximum SNR of $\frac{||\hbf||^2P_s }{P_\eta}$. Note that the optimal beamforming weights is dependent on the multi-path channel taps.

Our goal is to show how it compares against the SNR of a single beam and our multi-beam system. We first write the channel in a geometric model representation~\cite{alkhateeb2014channel,sayeed2007maximizing}:
\begin{equation}
    \begin{split}
        \hbf(t) =\sum_{\ell=0}^{L-1} \abf (\phi_\ell) \gamma_\ell e^{2\pi f_c \tau_\ell}\delta(t-\tau_\ell),
    \end{split}
\end{equation}
where we assume the channel is bounded by $L$ paths and $\phi_\ell, \gamma_\ell, \tau_\ell$ represents the AoD, attenuation, and ToF of the $\ell^{th}$ path, respectively. The steering vector $\abf (\phi_\ell)$ represents the relative phase shift introduced by each path at every antenna element (out of $N $ elements) as  $$ \textbf{a} (\phi_\ell) =[1,e^{-j2\pi\frac{d}{\lambda}\sin(\phi_\ell)},\ldots,e^{-j2\pi(N -1)\frac{d}{\lambda}\sin(\phi_\ell)}]^T$$

In the frequency domain, the channel is written at subcarrier $k$ as follow:
\begin{equation}
    \begin{split}
        \hbf(k) = \sum_{\ell=0}^{L-1} \abf (\phi_\ell) \gamma_\ell e^{j 2\pi (f_c +k \Delta f) \tau_\ell} 
        % \approx \sum_{\ell=0}^{L-1} \abf (\phi_\ell) \gamma_\ell e^{j 2\pi f_c \tau_\ell},
    \end{split}
\end{equation}
where $f_c$ is center frequency and $\Delta f$ is the subcarrier spacing. 
% The approximation follows since the center frequency of 28 GHz is much higher compared to the bandwidth of even 400 MHz.

The traditional single-beam pattern ignores the multi-path and creates a directional pattern along the strongest path (LOS or one of the reflectors). Assuming $\phi_0$ is the direction of the strongest path, the single-beam antenna weights follows:
\begin{equation}
\begin{split}
     \wbf ^{\text{single}}  &= \abf ^*(\phi_0)/||\abf (\phi_0)|| \\
     &= \frac{1}{\sqrt{N }}[1, e^{j2\pi \frac{d}{\lambda}\sin(\phi_0)},\ldots,  e^{j2\pi(N-1) \frac{d}{\lambda})\sin(\phi_0)}]^T.
\end{split}
\end{equation}

Assuming a directional single-beam pattern severely attenuates other channel paths, the single-beam SNR consists only of the strongest path as:
\begin{equation}
    \text{SNR}^{\text{single}} = \frac{||\gamma_0||^2P_s }{P_\eta}.
\end{equation}
Instead, we design phase-coherent multi-beam patterns which exploits $B$ channel directions out of $L$ paths as follow: 
\begin{equation}
    \wbf ^{\text{multi}} = \frac{\sum_{b=0}^{B-1} \abf ^*(\phi_b) \gamma_b e^{j  \sigma_b}}{||\sum_{b=0}^{B-1} \abf ^*(\phi_b) \gamma_b e^{j  \sigma_b}||},
\end{equation}
where we orient all the $B$ beams in the multi-beam along the $B$ strongest paths in the channel. Note that our multi-beam patterns ensures that per-beam amplitude $\gamma_b$ and phase $ \sigma_b$ (averaged over all frequency subcarriers) is aligned with per-path channel attenuation and phase respectively. We clearly see that when $B=L$, i.e., the multi-beam patterns are oriented along all the paths in a multi-path channel. In this case, the multi-beam weights are same as the optimal weights in (\ref{eq:wmrc2}):
\begin{equation}
     \wbf ^{\text{multi}} = \wbf ^{\text{opt}}, \quad \text{ when } B=L.
\end{equation}

Thus, a multi-beam pattern utilizes $B$ out of $L$ channel paths to improve the SNR as follows:
\begin{equation}
    \text{SNR}^{\text{multi}} = \frac{\sum_{b=0}^{B-1}||\gamma_b||^2P_s}{P_\eta},
\end{equation}
which converges to optimal SNR for $B=L$. We can write the capacity of multibeam-link as
\begin{equation}
    C_{mb} = \log_2(1+\text{SNR}^{\text{multi}})
\end{equation}
The optimal ML beamformer requires per-antenna channel estimate which has a high complexity in terms of beam probing overhead~\cite{palacios2018adaptive}.  \textit{Since mmWave channel is sparse and there are only 1 or 2 strong reflected paths in addition to the direct path, the multi-beam with 2-3 beams provides SNR gain comparable to the optimal beam with significantly lower overhead.}

 \begin{figure}[h]
\subfigure[]{\includegraphics[width=0.21\textwidth]{figures/wirelessInsite.pdf}\label{fig:wirelessInsite}}
\subfigure[]{\includegraphics[width=0.25\textwidth]{figures/compare28and60.pdf}\label{fig:compare28and60}}
\caption{(a) Wireless Insite simulation scenario, (b) Throughput Gain comparing 28 GHz and 60 GHz system for static UE with 10\% blockages.}
\label{fig:wi60ghz}
\end{figure}
\review{The experimental setup is at 28 GHz as opposed to the 60 GHz band. While I understand the hardware limitations of building a large phased array platform at 60 GHz, it is not completely clear whether the results at 28 GHz perfectly translate to 60 GHz since signal propagation characteristics are quite different.}

\section{Comparing \constructivemultibeam performance for 28 GHz and 60 GHz links}\label{sec:60ghz}
\name presents a general framework to improve mmWave throughput and reliability that can also be applied to a 60 GHz link. To compare the two systems, we perform a simulation study using Wireless Insite \cite{wirelessinsite}, as shown in Figure \ref{fig:wi60ghz}. We establish a directional link at 10m with a reflecting surface (made up of concrete material) at $60^o$ (Figure \ref{fig:wirelessInsite}). We set other simulation parameters according to a recent large-scale study of a 60 GHz system~\cite{wang2020demystifying}. The results in Fig.~\ref{fig:compare28and60} show that \name outperforms single-beam based baseline \cite{sur2016beamspy} by 1.18$\times$ gain in throughput for static UE with 10$\%$ blockages. Both 28 GHz and 60 GHz system performs similarly, and the result is consistent across multiple UE locations. Nonetheless, 28 GHz throughput is $4.7\times$ higher than 60 GHz (not shown) for the same bandwidth since 60 GHz links suffer from higher path loss and attenuation due to environmental absorption.
Though 28 GHz performance is better for longer links (AOD $\ge 15^o$) since 60 GHz links suffer from larger path loss and attenuation due to atmospheric absorption.
