# Supplementary material for: CommRad: Context-Aware Sensing-Driven Millimeter-Wave Networks
Source: arXiv:2407.08817 source file (2024-07-11)
Supplement: Supplementary file 2 [file sigcomm21_artifact_appendix_template.tex]

%%%%%%%%%%%%%%%%%%%%%%%%%%%%%%%%%%%%%%%%%%%%%%%%%%%%
% This part is included to make the appendix compilable as a standalone document.
% \documentclass{article}
% \usepackage{hyperref}
% \begin{document}
% %%%%%%%%%%%%%%%%%%%%%%%%%%%%%%%%%%%%%%%%%%%%%%%%%%%%

% \appendix
\section{Artifact Appendix}

\subsection*{Abstract}

{\em Required. Provide a short description of your artifact.}

\subsection*{Scope}

{\em Required. Explain what claims the artifact allows to validate and for what purposes it can be used.}

\subsection*{Contents}

{\em Required. Explain the contents of the artifact.}

\subsection*{Hosting}

{\em Required. Explain how to obtain the artifact. Be specific. If you host the artifact on GitHub, please mention the name of the branch and commit version. You might also want to consider hosting your repository on a platform like Zenodo, which assigns a unique DOI and is integrated \href{https://guides.github.com/activities/citable-code/}{well with GitHub}.}

\subsection*{Requirements}

{\em Required. Explain any special hardware or software requirements, or state the platform on which the artifact has been developed and tested.}

\subsection*{\ldots{}}

{\em Optional. Below the sections above, you can add any number of additional sections that are specific to your artifact.}


%%%%%%%%%%%%%%%%%%%%%%%%%%%%%%%%%%%%%%%%%%%%%%%%%%%%
% This part is included to make the appendix compilable as a standalone document.
% \end{document}
%%%%%%%%%%%%%%%%%%%%%%%%%%%%%%%%%%%%%%%%%%%%%%%%%%%%
